# Supplementary material for: Weak anti-localization and spin-momentum locking in topological insulator Ta$_2$Ni$_3$Te$_5$
Source: arXiv:2406.07864 source file (2024-06-12)
Supplement: Supplementary file 1 [file supplementary_Ta2Ni3Te5.pdf]

# Supplementary Section:

# Weak anti-localization and spin-momentum locking in topological insulator $Ta_2Ni_3Te_5$

Prabuddha Kant Mishra,[1] Soumen Ash,[1,*] and Ashok Kumar Ganguli[1,2,†]

[1]*Department of Chemistry, Indian Institute of Technology Delhi, New Delhi 110016, India*

[2]*Department of Materials Science and Engineering, Indian Institute of Technology Delhi, New Delhi 110016, India*

# I. EXPERIMENTAL DETAILS

The most relevant and significant data have been shown and discussed in the main manuscript. Here, we have provided minor details about experimentation and analysis. In addition, we have shown data supporting the outcomes of the main manuscript. It consists of details related to following

A. Four-probe configuration

B. Magnetotransport studies

C. Magnetic studies

## A. Four-probe configuration

The contact for four probe resistivity measurement are as shown in the Fig. S1(a). The fine copper wire (dia $\approx$ 0.1 mm) was used for contact formation through silver paste which acts as an adhesive. A rectangular pellet of $Ta_2Ni_3Te_5$ having dimensions of 6 mm $\times$ 4 mm $\times$ 0.6 mm, was used for transport property measurements. As depicted in the figure, the outer terminals are for current and voltage measurements have been performed through inner terminals. In the configuration, the voltage contacts are separated apart by a distance of 3 mm. As discussed in the main manuscript, the magnetoresistance measurements have been performed in two distinct configurations depending upon the relative orientation of current and applied magnetic field directions. In configuration (1) the applied field is perpendicular to the current direction while in other configuration (2) both are in the same direction, depicted as (a) and (b) in the Fig. S1(a), respectively. The measurements have been carried out with an applied current of 10 mA and ac-frequency of 17 Hz in a lock-in technique for improved signal-noise ratio.

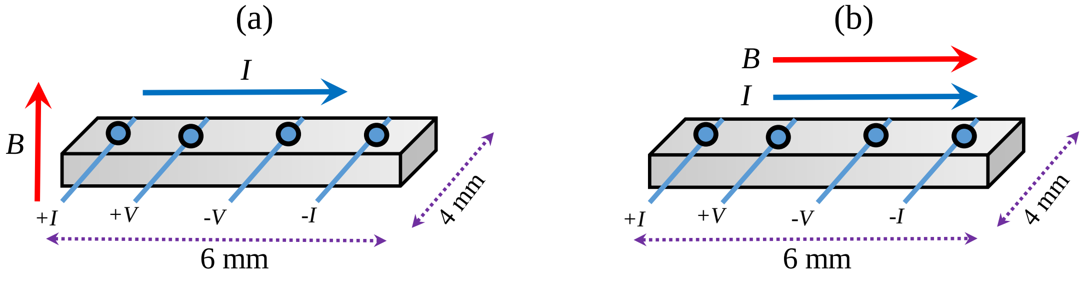


Figure 1. (Color online) The four-probe configurations for magnetoresistance measurements.


* Current Affiliation: Leibniz Institute for Solid State and Materials Research Dresden, 01069 Dresden, Germany.

† E-mail: ashok@chemistry.iitd.ac.in

### B. Magnetotransport studies

The magnetotransport has been performed at various temperatures and has significant values (40 % at $T$= 2 K) at low temperatures, as shown in the main manuscript. The origin of such a large response has been discussed as a topological feature, which gets diminished with an increase in the temperature resulting in a decrease in magnitude at elevated temperatures. Moreover, to minimize the geometry effect in the measured data of the Hall bar sample, we have used $\rho = [\rho(B) + \rho(-B)]/2$. The obtained summarized data with nullified Hall response has been shown in the figures.

Now, the MR data at various other temperatures (8 K $< T <$ 15 K) have been reordered for configuration $B \perp I$ and shown in the Fig. S2(a). The MR data at $T$ = 15 K have been fit with equation $A + cB^2$ as shown by the red curve in the Fig. S2(b). The parabolic field dependence of MR is associated with the trivial cyclotronic motion of electrons suggesting MR response in the high-temperature regime is dominated by bulk states. Further, an increase in temperature leads to decreased MR as shown in the Fig. S2(b).

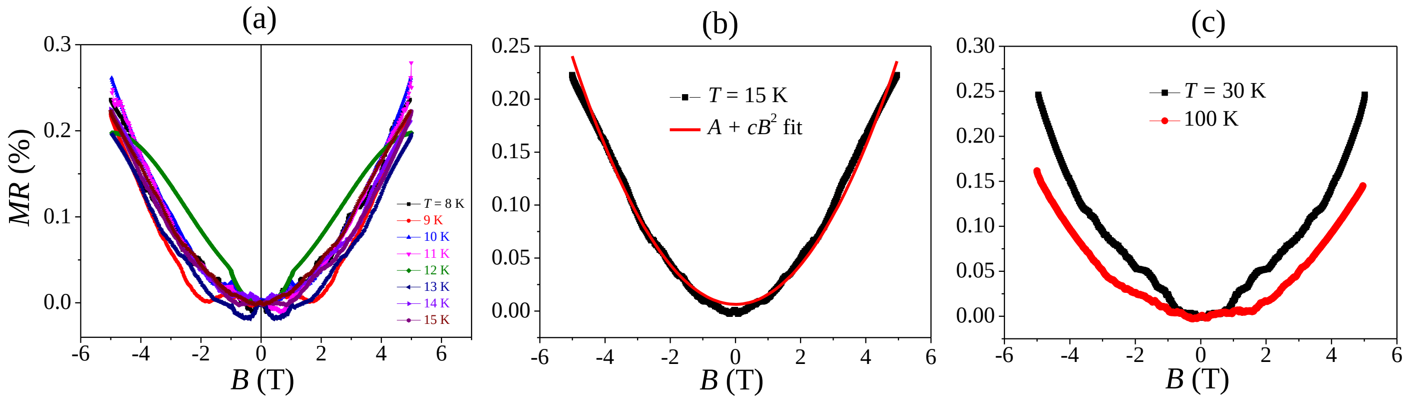


Figure 2. (Color online) (a) The magnetoresistance at temperatures (8 K $< T <$ 15 K) as function of applied field in the range of ± 5 T. (b) The parabolic beahviour for MR at 15 K, the red curve shows the $B^2$ fit. (c) MR data at elevated temperatures.

### C. Magnetic studies

As discernible from Fig. S2(a), we have measured the magnetization as a function of temperature for various applied fields under two protocols mainly. **(1). ZFC (Zero field cooled):** To record data as ZFC protocol, the sample has been cooled up to the desired temperature under zero applied magnetic field and data have been recorded while warming for a stable applied field. **(2). FC (Field cooled):**

In FC protocol, the magnetic field is applied during all the measurements, the sample is cooled under an applied magnetic field and data is recorded while warming.

The isothermal magnetization data at different temperatures have been recorded and have shown in the Fig. S3. For the measurements, the sample was cooled from high temperature ($T$= 100 K) to desired temperature under ZFC protocol and isothermal magnetization have been measured as function of applied field.

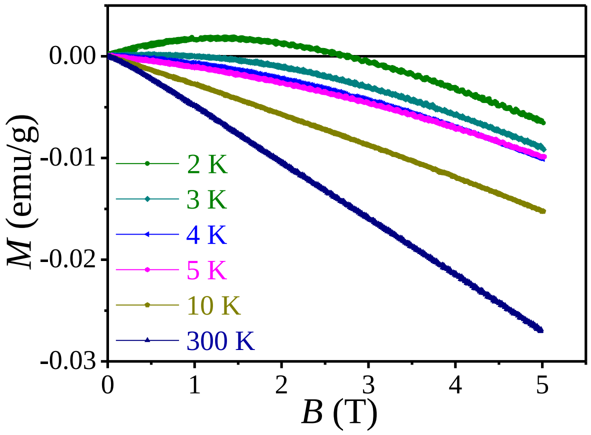


Figure 3. (Color online) (a) The isothermal magnetization data as function of function of field in the range of 0-5 T, at different temperatures.
